# Supplementary material for: SPAMs: Structured Implicit Parametric Models
Source: arXiv:2201.08141 source file (2022-01-20)

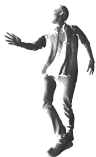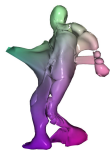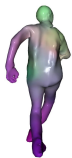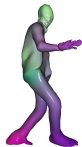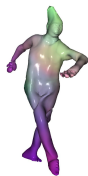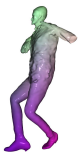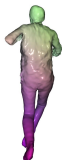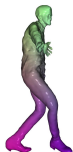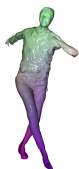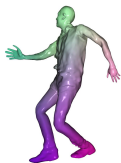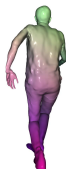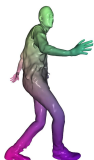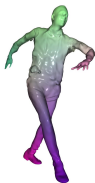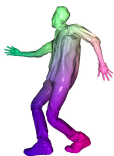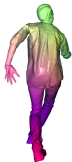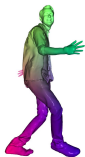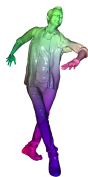

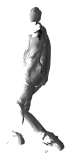

2.

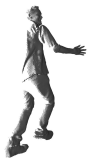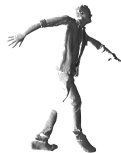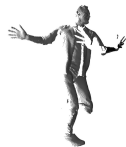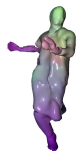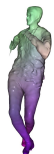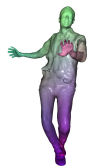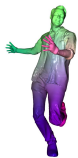

Supplement: Supplementary file 1 [file comparison_suppl.pdf]
